# Supplementary material for: Unified 3D Mesh Recovery of Humans and Animals by Learning Animal Exercise
Source: arXiv:2111.02450 source file (2021-11-03)
Supplement: Supplementary file 1 [file supp_compare.tex]

\begin{figure*}[h]
\centering
    \includegraphics[width=\linewidth]{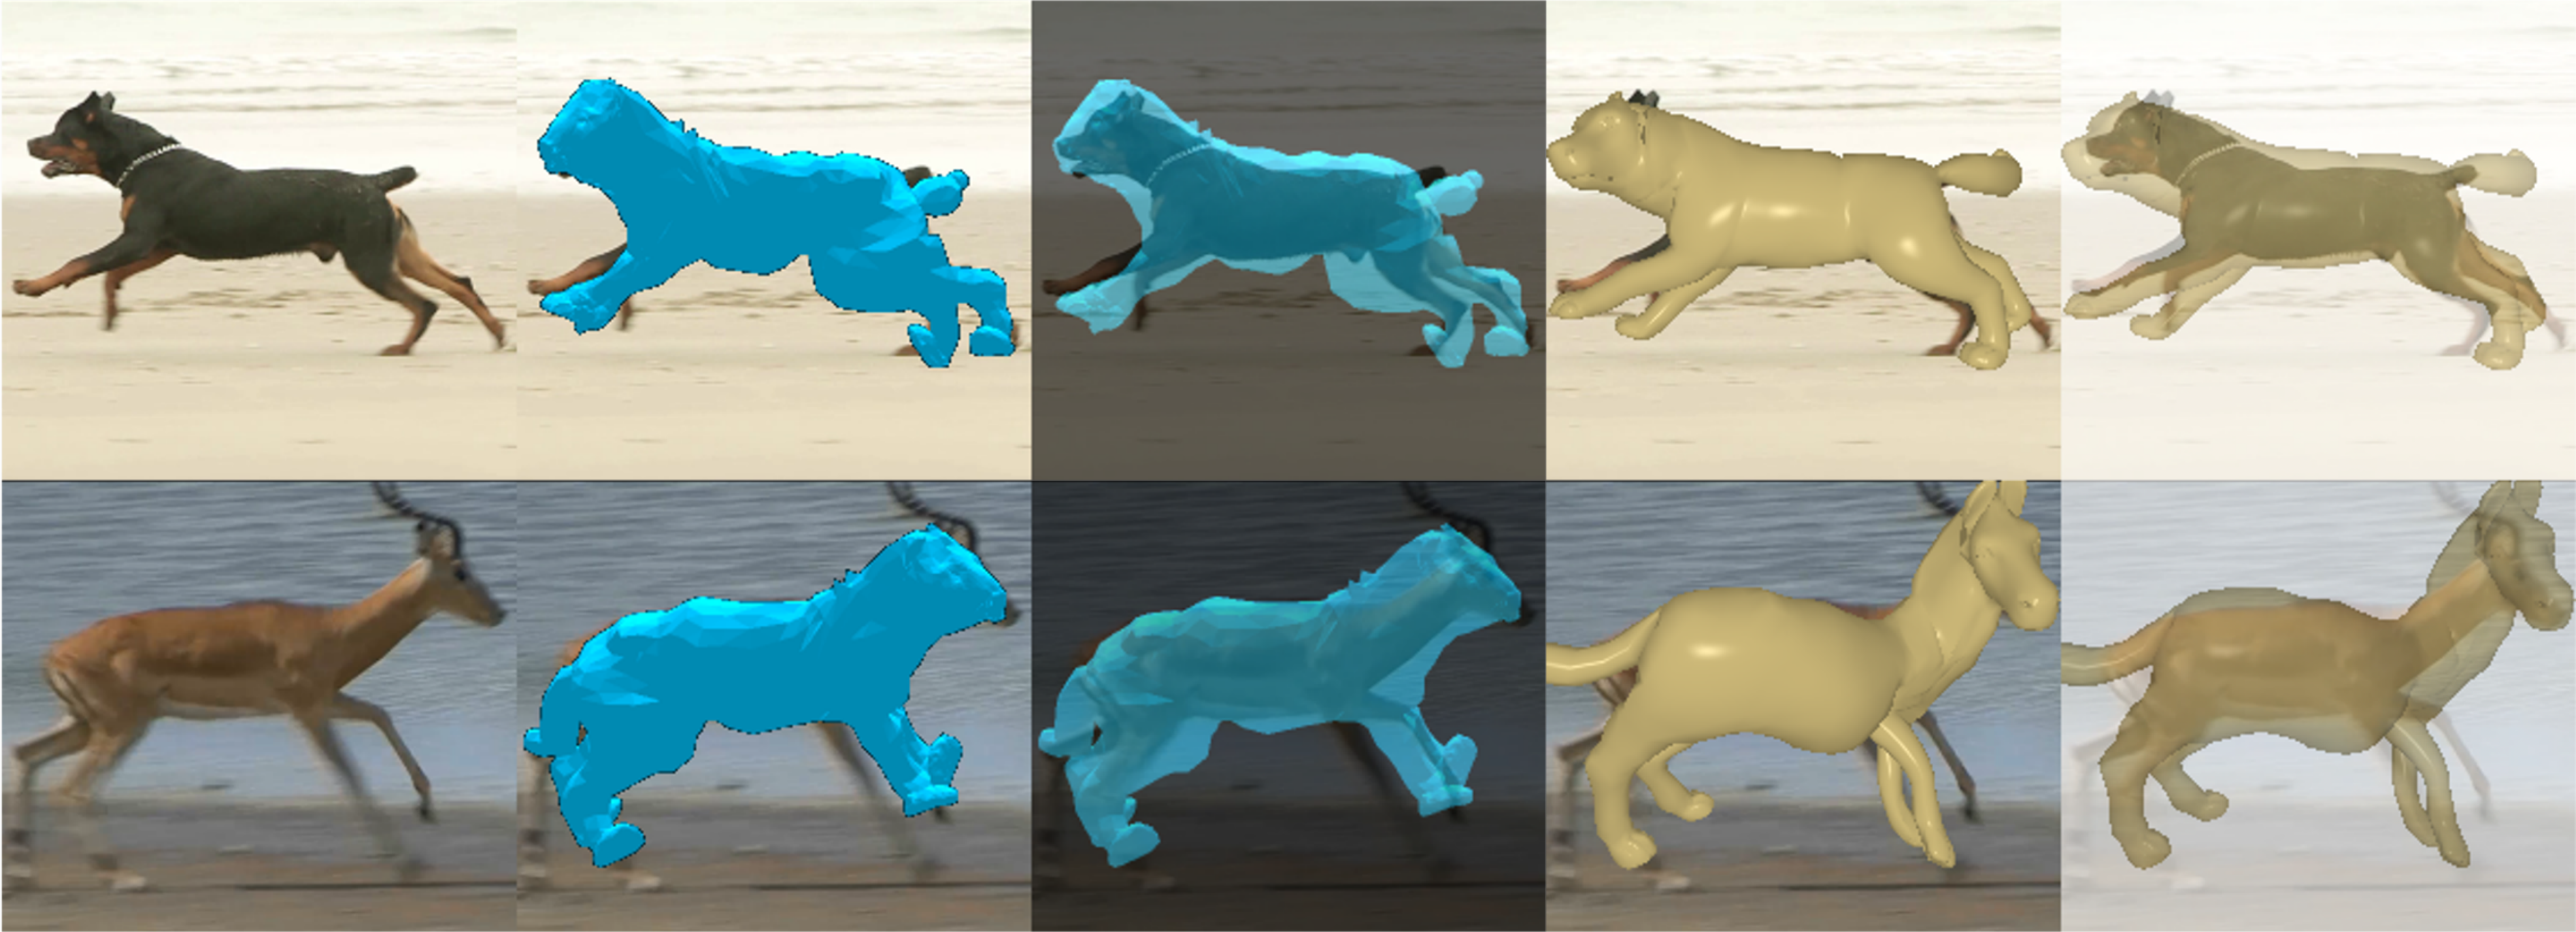}
\vspace{0.5mm}
\caption{\textbf{Comparison with WLDO}. Each column shows the input image, WLDO's mesh prediction~(blue), WLDO's mesh silhouette, \DeMR's mesh prediction~(yellow), \DeMR's mesh silhouette for BADJA: rs\_dog sequence (Top row), and for BADJA: impala0 sequence (Bottom row).}
% (Top row) Original image, WLDO's mesh prediction, WLDO's mesh silhouette, \DeMR's mesh prediction, \DeMR's mesh silhouette for BADJA-rs\_dog sequence. (Bottom row) Original image, WLDO's mesh prediction, WLDO's mesh silhouette, \DeMR's mesh prediction, \DeMR's mesh silhouette for BADJA-impala0 sequence.
% } 
% The first column shows original image. Column 2-3 (\oh{Blue}) shows the predicted meshes and projected mesh silhouettes for WLDO~\cite{biggs2020wldo}. Column 4-5 (Yellow) shows the \DeMR's mesh prediction result and projected mesh silhouette. 
% (Top row) BADJA-rs_dog sequence (Bottom row) Impala}
\vspace{-4.5mm}
    \label{fig:supp_comp}
\end{figure*}
