# Supplementary material for: Unified 3D Mesh Recovery of Humans and Animals by Learning Animal Exercise
Source: arXiv:2111.02450 source file (2021-11-03)
Supplement: Supplementary file 5 [file supp_subkpt.tex]

% \begin{wrapfigure}{R}{0.5\textwidth}
\begin{figure*}[h]
\centering
    \subfigure[]{\includegraphics[width=0.25\linewidth]{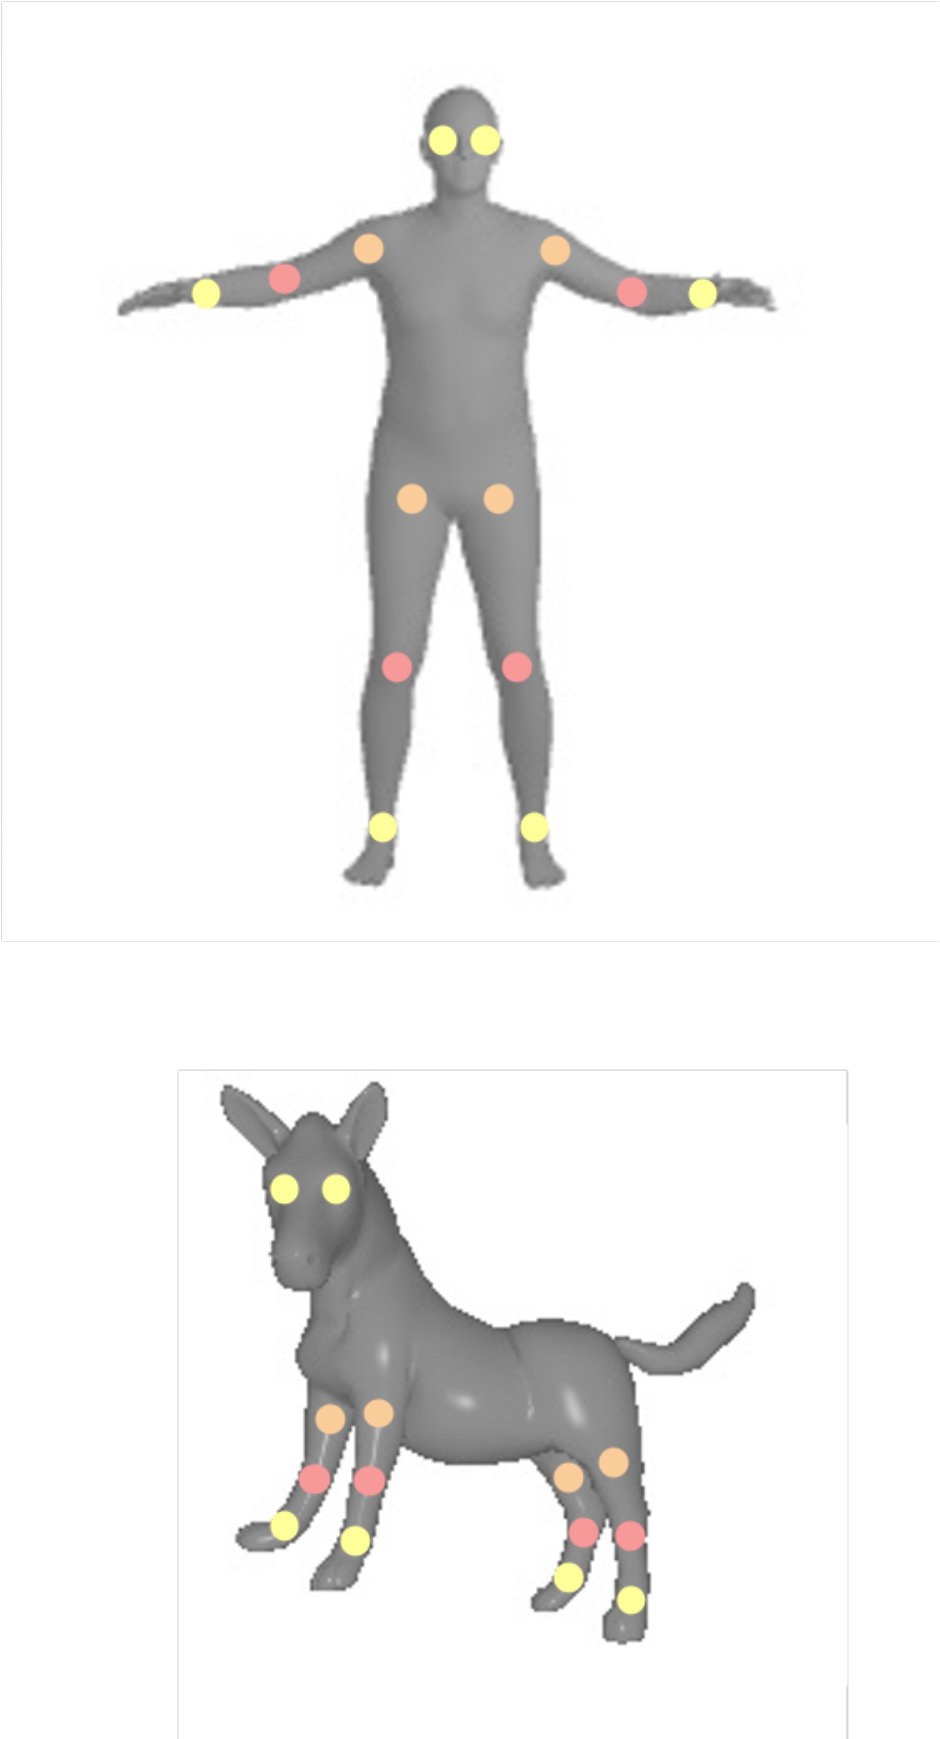}}
    \hspace{0.5cm}
    \subfigure[]{\includegraphics[width=0.25\linewidth]{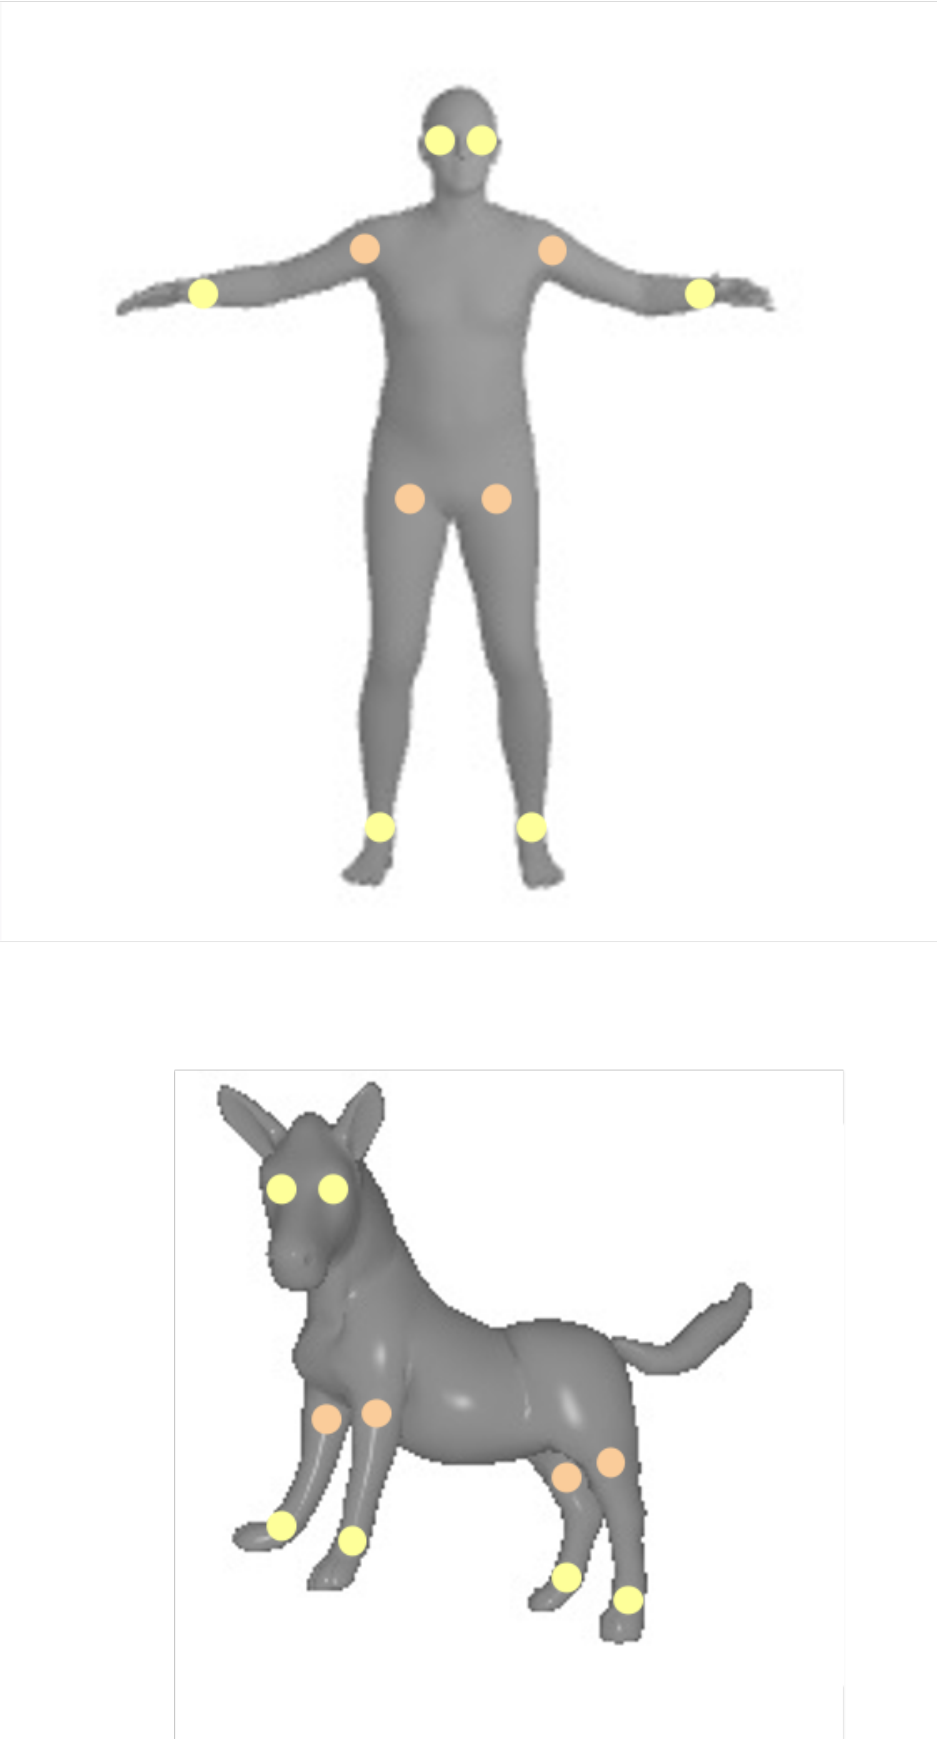}}
    \hspace{0.5cm}
    \subfigure[]{\includegraphics[width=0.25\linewidth]{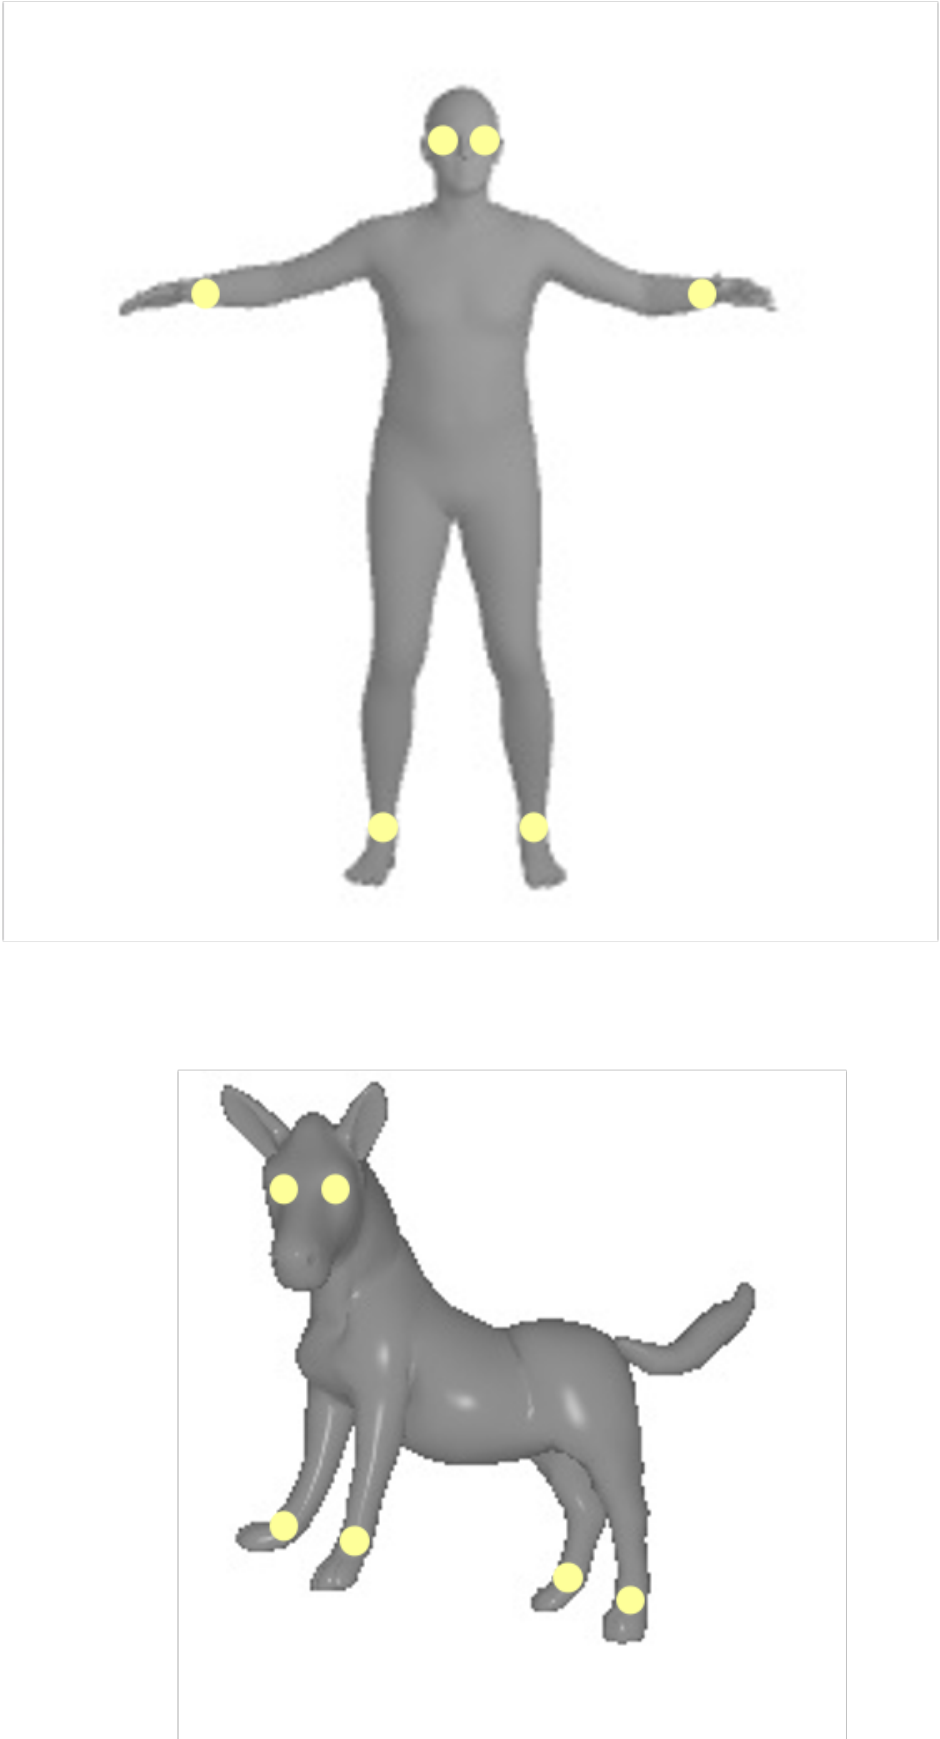}}
\vspace{3mm}
\caption{\textbf{Sub-keypoint settings}. (a) 15 sub-keypoints setting, including \{\emph{Eyes, Nose, TL, ML, BL}\}. (b) 10 sub-keypoints setting (Ours), including \{\emph{Eyes, Nose, TL, BL}\}. (c) 6 sub-keypoints setting, including \{\emph{Eyes, BL}\}. Best viewed in color.}
\vspace{-6mm}
\label{fig:supp_subkpt}
\end{figure*}
% \end{wrapfigure}
